# Supplementary material for: In-depth analysis of music structure as a text network
Source: arXiv:2303.13631 source file (2024-01-02)
Supplement: Supplementary file 1 [file supp.pdf]

# Supplemental Material: In-depth analysis structure of music via organizational essential element network

Ping-Rui Tsai<sup>1</sup>, Yen-Ting Chou<sup>1</sup>, Nathan-Christopher Wang<sup>2</sup>, Hui-Ling

Chen<sup>3</sup>, Hong-Yue Huang<sup>1</sup>, Zih-Jia Luo<sup>4</sup> and Tzay-Ming Hong<sup>1\*</sup>

<sup>1</sup>*Department of Physics, National Tsing Hua University, Hsinchu 30013, Taiwan, R.O.C*

<sup>3</sup>*College of Pharmacy, University of Michigan, Ann Arbor, MI 48109 U.S.A.*

<sup>2</sup>*Department of Chinese Literature, National Tsing Hua University, Hsinchu 30013, Taiwan, R.O.C and*

<sup>4</sup>*Advanced Semiconductor Engineering, INC., Kaohsiung 76027628, Taiwan, R.O.C*

## I. ESSENTIAL ELEMENT NETWORK

Our piano music samples encompass a range of periods in the history of Western classical music, from the earliest Baroque period (B), featuring the works of renowned composers such as Johann Sebastian Bach, Johann Pachelbel, and George Friedrich Handel, to the Classical period (BN) characterized by the music of composers such as Beethoven, and the Romantic period (R), which includes the works of composers such as Robert Alexander Schumann, Fryderyk Franciszek Chopin, and Achille-Claude Debussy, among others. Additionally, our collection includes modern Japanese music from composers such as Ryuichi Sakamoto and Joe Hisaishi.

In EEN, we set the range for scale and time weights to be 0.05 to 0.3 with an interval of 0.05 and the range for volume to be 0.1 to 0.4 with an interval of 0.1. We also normalized the decibel values between 0 and 10 for all data points. The threshold range was set to be 0.5 to 1.8 with an interval of 0.2. Our goal was to find the weights and threshold that would result in a Zipf's Law distribution of clustering coefficients with an R-squared value of 0.8 after deleting the first rank and taking the  $\log_{10}$  of the frequency on the y-axis and the word ranking on the x-axis, while also extracting the maximum number of diverse word types. While it is possible to use a gradient descent method to train the weights and calculate the self-organization between points, the model contains non-differentiable elements such as ranking word frequency, and the training time for songs longer than 3 minutes would take approximately 12 hours. Therefore, we used an exhaustive method with parallel computing.

## II. MINING MUSICAL TEXTS

If CC is calculated by scanning all time points from the first to the last scale, we can obtain a sequence with periodic characteristics. The Baroque period and the ambient sound are shown to share the same trend, as opposed to the Romantic period which adopts more diverse words to make the musical form in Fig. 1 which shows the histogram of Fig. 3(c) in the main text.

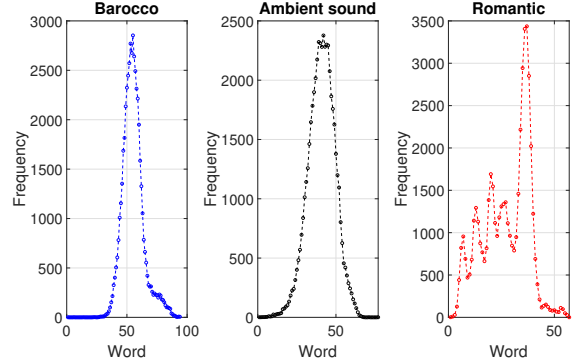

FIG. 1. Histograms for three types of music. Both Baroque and ambient sound observe a normal distribution of word clustering coefficient, while the Romantic period does not.

## III. DEEP LEARNING DETAILS FOR FIG. 4

In training, we had 34000/32456 samples for each of the three periods in Fig. 4(a) and (b) of the main text. However, due to the numerous CNNs used in training, we will only provide the minimum amount of information for Fig. 4(a), which includes the learning curve of (1) 2-scale and 2-second and (2) 72-scale and 3.5-second 2D EEN. Figures 2(a,b) and 2(c) correspond to the learning curve for Fig. 4(a) and 4(b) in the main text. All the CNN adopted four convolutional layers of 2\*2 kernel size and three fully connected layers with 128, 64, and 3 nodes, respectively, to complete the training. The hyperparameters used are: training-validation-test ratio of 6:2:2, batch size of 64, epoch of 6, and a learning rate of  $10^{-4}$ . The test accuracy for Fig. 4(b-d) in the main text is 0.93.

## IV. DEEP LEARNING DETAILS FOR FIG. 5

In training, there are 12,000 samples for both music and non-music. We used convolutional layers of 2\*2 kernel size and three fully connected layers with 128, 64, and 3 nodes, respectively, to complete the training. The hyperparameters used are: training-validation-test ratio of 6:2:2, batch size of 64, epoch of 6, and a learning rate of  $10^{-4}$ . The results are shown in Fig. 3 with the test accuracy equaling 1.

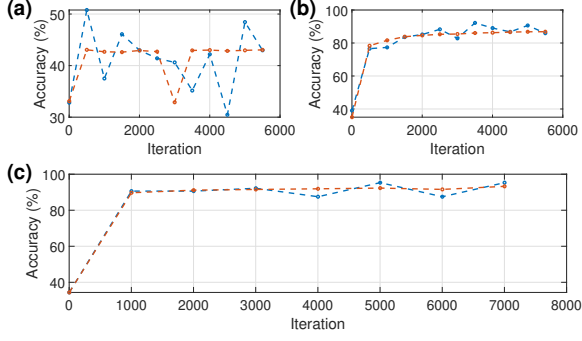

FIG. 2. The learning curves in (a,b) and (c) are for Fig. 4(a) and (b) in the main text, where the blue/orange dashed line denotes the training/validation accuracy.

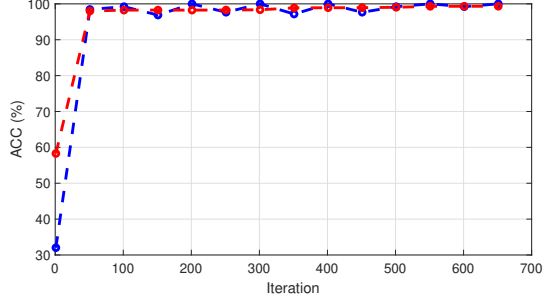

FIG. 3. The learning curves for Fig. 5(a, b) in the main text, where the blue/red dashed lines denote the training/validation accuracy.

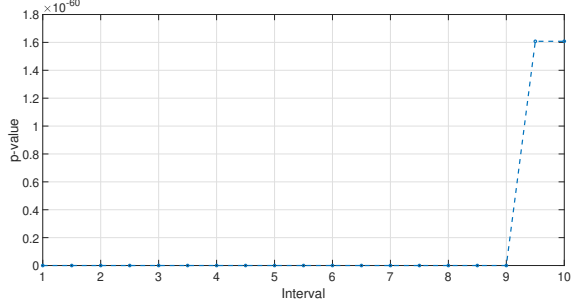

FIG. 4. The t-test for the density of Fig. 5(b) in the main text.

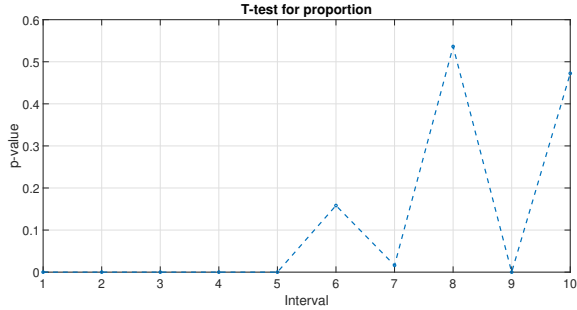

FIG. 5. The t-test for the proportion of Fig. 5(b) in the main text.

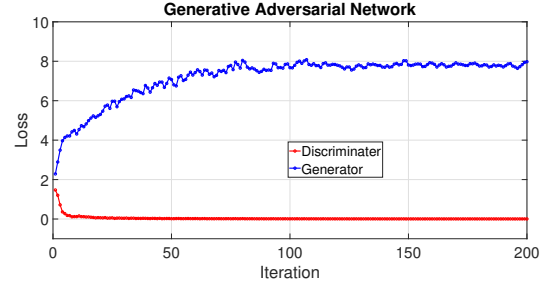

FIG. 6. The learning curve for the GAN of 1000 2D EEN images in Baroque and Romantic periods.

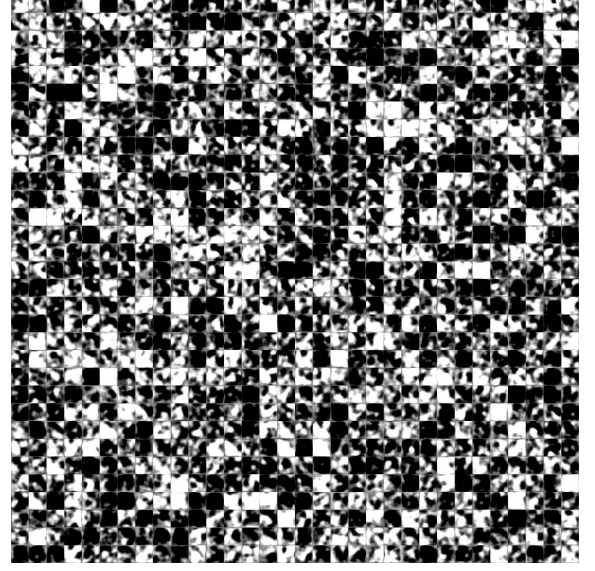

FIG. 7. The generated 2D EEN images by GAN.

## V. T-TEST FOR FIG. 5(B)

Complementing Fig. 5(b) for music and non-music at different intervals in the main text, the t-test results for the density and proportion are shown in Figs. 4 and 5.

## VI. GENERATIVE ADVERSARIAL NETWORK

We used 1000 2D EEN images for the Baroque period to create two generative adversarial networks. The batch size was 64, the image size was compressed to  $64 \times 64$ , and the epoch was set to 0.001. The learning curve is shown in Fig. 6, and the generated images are in Fig. 7.
